# Supplementary material for: Multidimensional coupling: A variationally consistent approach to fiber-reinforced materials
Source: arXiv:2101.02527 source file (2021-04-10)
Supplement: Supplementary file 1 [file sec_appendix1.tex]

\section{Proof of Proposition~\ref{th:condensed_sys}}\label{app:proof}
\begin{proof}[Proof of Proposition~\ref{th:condensed_sys}]
Using~\eqref{eq:sys:loads} with test functions~$\delta\fib{\vec{\varphi}} = \delta\vec{\varphi}|_{\mathfrak{C}_0}$,  we obtain~\eqref{eq:sys:matrix}.  Hence, after integration by parts and noting that $\partial_s \equiv \vec{D}_3\cdot\nabla$ and the endpoint conditions $\mathfrak{n} = \vec{n}_{ext}^{e}$ at $s=0,L$, we obtain
	\begin{equation}\label{eq:new:sys:matrix_condense}
	\begin{aligned}
	&\int\limits_{\mtx{\Omega}_0} \left(\drv{\mtx{\Psi}}{\ten{\mtx{F}}}:\nabla\delta\vec{\mtx{\varphi}}- \vec{B}_{ext}\cdot\delta\vec{\varphi}\right) \d V
	-
	\int\limits_{\Gamma^{\sigma}} \vec{T}_{ext}\cdot\delta\vec{\mtx{\varphi}} \d A
	\\
	&
	+\int\limits_{\mathfrak{C}_0}\left(\left[\mathfrak{n}\otimes\vec{D}_3\right] : \nabla\delta\mtx{\vec{\varphi}}
	-
	\bar{\tilde{\vec{n}}} \cdot \delta\mtx{\vec{\varphi}}\right)\d s
	-
	\EC{\vec{n}_{ext}^{e}\cdot\delta\mtx{\vec{\varphi}}} 
	\\&+
	\int\limits_{\mathfrak{C}_0}
	\frac{1}{2}\,\ten{\Sigma}:\nabla\delta\mtx{\vec{\varphi}} \abs{C}\d s
%	+
%	\EC{\frac{1}{2}\,\ten{\Sigma}^{e}: \nabla\delta\mtx{\vec{\varphi}}} \abs{A}
	= 0.
	\end{aligned}
	\end{equation}
Thus, we have eliminated the set of Lagrange multipliers $\bar{\vec{\mu}}$. For the second set of Lagrange multipliers~$\ten{\Sigma}$, we integrate in~\eqref{eq:sys:moments} with the test functions~$\delta\vec{\phi}= \ten{\mathcal{P}}_{\alpha}\tp\,\nabla\delta\vec{\mtx{\varphi}} \,\vec{D}_{\alpha} \in\L{2}(\mathfrak{C}_0)$. Taking the decomposition~\eqref{eq:PQ_decomp} and Lemma~\eqref{th:R2F} into account,  yields
	\begin{equation}\label{eq:expl_stress}
	-\int\limits_{\mathfrak{C}_0}\left[\ten{\mathcal{P}}_{\alpha}
	\left({\mathfrak{m}}^{\prime} + \tilde{\vec{\varphi}}^{\prime}\times{\mathfrak{n}}+\bar{\tilde{\vec{m}}}\right)
	\otimes\vec{D}_{\alpha}
	+
	\left(\ten{\Sigma}
	-
	\ten{F}_{c}\,[\tilde{\vec{\mu}}_n]_s
%	\ten{\mathcal{Q}}_{\alpha}\,\tilde{\vec{\mu}}_n\otimes\vec{D}_{\alpha}
	\right)	\abs{C}	
	\right]
	:
	\nabla\delta\vec{\mtx{\varphi}}
	\d s
	= 0.
	\end{equation}
Then, multiplying the above equation by $\frac{1}{2}$, adding it to~\eqref{eq:new:sys:matrix_condense} and integrating it by parts with the endpoint conditions $\mathfrak{m} = \vec{m}_{ext}^{e}$  at $s=0,L$, we obtain
	\begin{equation}\label{eq:new:sys:matrix_very_condense}
	\begin{aligned}
	&\,\int\limits_{\mtx{\Omega}_0} \biggl(\underbrace{\drv{\mtx{\Psi}}{\ten{\mtx{F}}}}_{\vec{P}}:\nabla\delta\vec{\mtx{\varphi}} - \vec{B}_{ext}\cdot\delta\vec{\varphi}\biggl) \d V 
	-
	\int\limits_{\Gamma^{\sigma}} \vec{T}_{ext}\cdot\delta\vec{\mtx{\varphi}} \d A
	\\
	&
	+
	\int\limits_{\mathfrak{C}_0}\biggl(\underbrace{\mathfrak{n}\otimes\vec{D}_3}_{\vec{P}^{\mathfrak{n}}} : \nabla\delta\mtx{\vec{\varphi}}
	-
	\bar{\tilde{\vec{n}}} \cdot \delta\mtx{\vec{\varphi}}\biggl)\d s  
	-
	\EC{\vec{n}_{ext}^{e}\cdot\delta\mtx{\vec{\varphi}}
		+
		\frac{1}{2}\left(\ten{\mathcal{P}}_{\alpha}\,\vec{m}_{ext}^{e} \otimes\,\vec{D}_{\alpha}\right):\nabla\delta\mtx{\vec{\varphi}}}
	\\
	&
	+\,
	\int\limits_{\mathfrak{C}_0}
	\underbrace{\frac{1}{2}\left[\ten{\mathcal{P}}_{\alpha}\,\mathfrak{m}\otimes\vec{D}_\alpha\otimes\vec{D}_3\right]}_{\mathfrak{P}}\,\vdots\,\nabla^2\delta\mtx{\vec{\varphi}}
	\d s
	+
	\int\limits_{\mathfrak{C}_0}
	\underbrace{\frac{1}{2}\left[\ten{\mathcal{P}}_{\alpha}\,\mathfrak{m}\otimes\vec{D}_\alpha^\prime\right]}_{\vec{P}^{g}}:\nabla\delta\mtx{\vec{\varphi}}
	\d s
	\\
	&+\,
	\int\limits_{\mathfrak{C}_0}
	\biggl(\underbrace{\frac{1}{2}\left[\ten{\mathcal{P}}_{\alpha}^\prime\,\mathfrak{m}
%		+ \ten{\mathcal{Q}}_{\alpha}\,\tilde{\vec{\mu}}_n
		-\ten{\mathcal{P}}_{\alpha}\left(\tilde{\vec{\varphi}}^{\prime}\times{\mathfrak{n}} +\bar{\tilde{\vec{m}}}\right)
		\right]\otimes\vec{D}_{\alpha}}_{\vec{P}^{\mathfrak{m}}}
		+
		\frac{1}{2}\,\ten{F}_{c}\,[\tilde{\vec{\mu}}_n]_s\,\abs{C}\biggr):\nabla\delta\mtx{\vec{\varphi}}\,\d s
	= 0,
	\end{aligned}
	\end{equation}
	supplemented with constitutive equations~\eqref{eq:constitutive_n}-\eqref{eq:constitutive_m} and coupling constraints \eqref{eq:sys:pi1}, \eqref{eq:coup_cond1} and \eqref{eq:area_cond_F}.
\end{proof}

\section{Parametrization of the rotation tensor in terms of quaternions}\label{app:quarternions}
Quaternions $\mathfrak{q} = (q_0,\vec{q})$ can be written in terms of the scalar part $q_0\in\mathbb{R}$ and the vector part $\vec{q}\in\mathbb{R}^3$. Restricting the quaternions to unit length, i.e., $|\mathfrak{q}| = 1$ such that we consider a unit sphere in $\mathbb{R}^4$, we form a group as
\begin{equation}
\mathcal{S}^3 = \{\mathfrak{q}\in\mathbb{R}^4|\; |\mathfrak{q}| = 1\},
\end{equation}
see \cite{betsch2009c} for details. This allows us to introduce a mapping $\tilde{\vec{R}}:\mathcal{S}^3\rightarrow SO(3)$
\begin{equation}
\tilde{\vec{R}}(\mathfrak{q}) = (q_0^2-\vec{q}\cdot\vec{q})\,\vec{I} + 2\,\vec{q}\otimes\vec{q} + 2\,q_0\,\hat{\vec{q}},
\end{equation}
called Euler-Rodrigues parametrization, see Marsden and Ratiu \cite{marsden2003}. 

\section{Rigid bodies}\label{app:Spherical}
If a Cosserat point instead of a Cosserat beam is taken into account, i.e.\ a 0D-3D coupling, we have to constraint the whole sphere instead of the cross section. With regard to \eqref{eq:new:mu_tilde}, we decompose $\tilde{\vec{\mu}}$ into torque and pressure
\begin{equation}\label{eq:lmDef}
\tilde{\vec{\mu}}(\theta^i) = \vec{\mu}_{\tau}\times\left[\tilde{\vec{R}}\,\vec{N}(\theta^i)\right] + \mu_n\,\tilde{\vec{R}}\,\vec{N}(\theta^i).
\end{equation}
Next we insert \eqref{eq:lmDef} in \eqref{eq:coupling_term_proof} and note that
\begin{equation}
\begin{aligned}
\left(\vec{\mu}_{\tau}\times\left[\tilde{\vec{R}}\,\vec{N}\right]\right)\cdot\left(\left[\vec{F}_c-\tilde{\vec{R}}\right]\theta^i\,\vec{D}_i\right) &= \left(\tilde{\vec{R}}\tp\,\vec{\mu}_{\tau}\right)\cdot\left[\vec{N}\times\left(\tilde{\vec{R}}\tp\,\left[\vec{F}_c-\tilde{\vec{R}}\right]\,\vec{N}\right)\right]\,\|\theta^i\,\vec{D}_i\|,\\
&= \left(\tilde{\vec{R}}\tp\,\vec{\mu}_{\tau}\right)\cdot\left[\vec{N}\times\left(\tilde{\vec{R}}\tp\,\vec{F}_c\,\vec{N}\right)\right]\,\|\theta^i\,\vec{D}_i\|.\\
\end{aligned}
\end{equation}
Making use of a spherical parametrization
\begin{equation}\label{key2}
\vec{N} = \vec{D}_1\,\cos\theta\,\sin\phi + \vec{D}_2\,\sin\theta\,\sin\phi + \vec{D}_3\,\cos\phi,
\end{equation}
we obtain for an arbitrary matrix~$\vec{A}$
	\begin{equation}
	\begin{aligned}
	&\int\limits_{0}^{2\pi}\int\limits_{-\pi}^{\pi} \vec{N}\times\bigl(\ten{A}\,\vec{N} \bigr)\,\d\theta\d\phi
	= \int\limits_{0}^{2\pi}\begin{vmatrix} \vec{D}_1 & \vec{D}_2 & \vec{D}_3 \\ 
	\cos\theta\,\sin\phi & \sin\theta\,\sin\phi & \cos\phi \\
	\vec{D}_1\tp\,\ten{A}\,\vec{N} & \vec{D}_2\tp\,\ten{A}\,\vec{N} & \vec{D}_3\tp\,\ten{A}\,\vec{N}
	\end{vmatrix}\,\d\theta 
	\\
	&= \left[\vec{D}_1,  \vec{D}_2,  \vec{D}_3\right]\cdot
	\int\limits_{0}^{2\pi}
	\begin{bmatrix} 
	\phantom{-}\vec{D}_3\tp\,\ten{A}\,\vec{N}\,\sin\theta\,\sin\phi - \vec{D}_2\tp\,\ten{A}\,\vec{N}\,\cos\phi\,\phantom{\cos\phi}\\ 
	-\vec{D}_3\tp\,\ten{A}\,\vec{N}\,\cos\theta\,\sin\phi  + \vec{D}_1\tp\,\ten{A}\,\vec{N}\,\cos\phi\,\phantom{\cos\phi}\\
	\phantom{-}\vec{D}_2\tp\,\ten{A}\,\vec{N}\,\cos\theta\,\sin\phi - \vec{D}_1\tp\,\ten{A}\,\vec{N}\,\sin\theta\,\sin\phi
	\end{bmatrix}\,\d\theta
	\\
	&=
	\pi\left[\vec{D}_1,  \vec{D}_2,  \vec{D}_3\right]\cdot\begin{bmatrix} 
	\phantom{-}\vec{D}_3\tp\,\ten{A}\,\vec{D}_2 - \vec{D}_2\tp\,\ten{A}\,\vec{D}_3 \\ 
	-\vec{D}_3\tp\,\ten{A}\,\vec{D}_1 + \vec{D}_1\tp\,\ten{A}\,\vec{D}_3\\
	\phantom{-}\vec{D}_2\tp\,\ten{A}\,\vec{D}_1 - \vec{D}_1\tp\,\ten{A}\,\vec{D}_2	
	\end{bmatrix} \\
	&=
	2\,\pi\,\left[\vec{D}_1,  \vec{D}_2,  \vec{D}_3\right]\cdot\axl\left(\left[\vec{D}_1,  \vec{D}_2,  \vec{D}_3\right]\tp\,\ten{A}\,\left[\vec{D}_1,  \vec{D}_2,  \vec{D}_3\right]\right),
	\end{aligned}
	\end{equation}
and thus
\begin{equation}
\int\limits_{0}^{2\pi}\int\limits_{-\pi}^{\pi} \vec{N}\times\bigl(\fib{\vec{R}}\tp\,\vec{F}_{c}\,\vec{N} \bigr)\,\d\theta\d\phi = 
2\,\pi\,\left[\vec{D}_1,  \vec{D}_2,  \vec{D}_3\right]\cdot\axl\left(\left[\vec{D}_1,  \vec{D}_2,  \vec{D}_3\right]\tp\,\fib{\vec{R}}\tp\,\vec{F}_{c}\,\left[\vec{D}_1,  \vec{D}_2,  \vec{D}_3\right]\right).
\end{equation}	
Finally, we can state
\begin{equation}
\skewsym\big(\left[\vec{D}_1,  \vec{D}_2,  \vec{D}_3\right]\tp\,\fib{\ten{R}}\tp\,\mtx{\ten{F}_{c}}\,\left[\vec{D}_1,  \vec{D}_2,  \vec{D}_3\right]\big)=
\left[\vec{D}_1,  \vec{D}_2,  \vec{D}_3\right]\tp\, \skewsym(\fib{\ten{R}}\tp\,\mtx{\ten{F}_{c}}) \,\left[\vec{D}_1,  \vec{D}_2,  \vec{D}_3\right],
\end{equation}	
i.e.,\ we have to enforce that $\skewsym(\fib{\ten{R}}\tp\,\mtx{\ten{F}_{c}})$ is zero. Note that this is equivalent to the formulation considered in \cite{simo1992h}.
