# Supplementary material for: Multidimensional coupling: A variationally consistent approach to fiber-reinforced materials
Source: arXiv:2101.02527 source file (2021-04-10)
Supplement: Supplementary file 2 [file sec_appendix.tex]

\begin{comment}

\section{Parametrization of the rotation tensor in terms of quaternions}\label{app:quarternions}
Quaternions $\mathfrak{q} = (q_0,\vec{q})$ can be written in terms of the scalar part $q_0\in\mathbb{R}$ and the vector part $\vec{q}\in\mathbb{R}^3$. Restricting the quaternions to unit length, i.e., $|\mathfrak{q}| = 1$ such that we consider a unit sphere in $\mathbb{R}^4$, we form a group as
\begin{equation}
\mathcal{S}^3 = \{\mathfrak{q}\in\mathbb{R}^4|\; |\mathfrak{q}| = 1\},
\end{equation}
see \cite{betsch2009c} for details. This allows us to introduce a mapping $\tilde{\vec{R}}:\mathcal{S}^3\rightarrow SO(3)$
\begin{equation}
\tilde{\vec{R}}(\mathfrak{q}) = (q_0^2-\vec{q}\cdot\vec{q})\,\vec{I} + 2\,\vec{q}\otimes\vec{q} + 2\,q_0\,\hat{\vec{q}},
\end{equation}
called Euler-Rodrigues parametrization, see Marsden and Ratiu \cite{marsden2003}. 

\end{comment}

\section{Rigid bodies}\label{app:Spherical}
If a Cosserat point instead of a Cosserat beam is taken into account, i.e.\ a 0D-3D coupling, we have to constraint the whole sphere instead of the cross section. With regard to \eqref{eq:new:mu_tilde}, we decompose $\tilde{\vec{\mu}}$ into torque and pressure
\begin{equation}\label{eq:lmDef}
\tilde{\vec{\mu}}(\theta^i) = \vec{\mu}_{\tau}\times\left[\tilde{\vec{R}}\,\vec{N}(\theta^i)\right] + \mu_n\,\tilde{\vec{R}}\,\vec{N}(\theta^i).
\end{equation}
Next we insert \eqref{eq:lmDef} in \eqref{eq:coupling_term_proof} and note that
\begin{equation}
\begin{aligned}
\left(\vec{\mu}_{\tau}\times\left[\tilde{\vec{R}}\,\vec{N}\right]\right)\cdot\left(\left[\vec{F}_c-\tilde{\vec{R}}\right]\theta^i\,\vec{D}_i\right) &= \left(\tilde{\vec{R}}\tp\,\vec{\mu}_{\tau}\right)\cdot\left[\vec{N}\times\left(\tilde{\vec{R}}\tp\,\left[\vec{F}_c-\tilde{\vec{R}}\right]\,\vec{N}\right)\right]\,\|\theta^i\,\vec{D}_i\|,\\
&= \left(\tilde{\vec{R}}\tp\,\vec{\mu}_{\tau}\right)\cdot\left[\vec{N}\times\left(\tilde{\vec{R}}\tp\,\vec{F}_c\,\vec{N}\right)\right]\,\|\theta^i\,\vec{D}_i\|.\\
\end{aligned}
\end{equation}
Making use of a spherical parametrization
\begin{equation}\label{key2}
\vec{N} = \vec{D}_1\,\cos\theta\,\sin\phi + \vec{D}_2\,\sin\theta\,\sin\phi + \vec{D}_3\,\cos\phi,
\end{equation}
we obtain for an arbitrary matrix~$\vec{A}$
	\begin{equation}
	\begin{aligned}
	&\int\limits_{0}^{2\pi}\int\limits_{-\pi}^{\pi} \vec{N}\times\bigl(\ten{A}\,\vec{N} \bigr)\,\d\theta\d\phi
	= \int\limits_{0}^{2\pi}\begin{vmatrix} \vec{D}_1 & \vec{D}_2 & \vec{D}_3 \\ 
	\cos\theta\,\sin\phi & \sin\theta\,\sin\phi & \cos\phi \\
	\vec{D}_1\tp\,\ten{A}\,\vec{N} & \vec{D}_2\tp\,\ten{A}\,\vec{N} & \vec{D}_3\tp\,\ten{A}\,\vec{N}
	\end{vmatrix}\,\d\theta 
	\\
	&= \left[\vec{D}_1,  \vec{D}_2,  \vec{D}_3\right]\cdot
	\int\limits_{0}^{2\pi}
	\begin{bmatrix} 
	\phantom{-}\vec{D}_3\tp\,\ten{A}\,\vec{N}\,\sin\theta\,\sin\phi - \vec{D}_2\tp\,\ten{A}\,\vec{N}\,\cos\phi\,\phantom{\cos\phi}\\ 
	-\vec{D}_3\tp\,\ten{A}\,\vec{N}\,\cos\theta\,\sin\phi  + \vec{D}_1\tp\,\ten{A}\,\vec{N}\,\cos\phi\,\phantom{\cos\phi}\\
	\phantom{-}\vec{D}_2\tp\,\ten{A}\,\vec{N}\,\cos\theta\,\sin\phi - \vec{D}_1\tp\,\ten{A}\,\vec{N}\,\sin\theta\,\sin\phi
	\end{bmatrix}\,\d\theta
	\\
	&=
	\pi\left[\vec{D}_1,  \vec{D}_2,  \vec{D}_3\right]\cdot\begin{bmatrix} 
	\phantom{-}\vec{D}_3\tp\,\ten{A}\,\vec{D}_2 - \vec{D}_2\tp\,\ten{A}\,\vec{D}_3 \\ 
	-\vec{D}_3\tp\,\ten{A}\,\vec{D}_1 + \vec{D}_1\tp\,\ten{A}\,\vec{D}_3\\
	\phantom{-}\vec{D}_2\tp\,\ten{A}\,\vec{D}_1 - \vec{D}_1\tp\,\ten{A}\,\vec{D}_2	
	\end{bmatrix} \\
	&=
	2\,\pi\,\left[\vec{D}_1,  \vec{D}_2,  \vec{D}_3\right]\cdot\axl\left(\left[\vec{D}_1,  \vec{D}_2,  \vec{D}_3\right]\tp\,\ten{A}\,\left[\vec{D}_1,  \vec{D}_2,  \vec{D}_3\right]\right),
	\end{aligned}
	\end{equation}
and thus
\begin{equation}
\int\limits_{0}^{2\pi}\int\limits_{-\pi}^{\pi} \vec{N}\times\bigl(\fib{\vec{R}}\tp\,\vec{F}_{c}\,\vec{N} \bigr)\,\d\theta\d\phi = 
2\,\pi\,\left[\vec{D}_1,  \vec{D}_2,  \vec{D}_3\right]\cdot\axl\left(\left[\vec{D}_1,  \vec{D}_2,  \vec{D}_3\right]\tp\,\fib{\vec{R}}\tp\,\vec{F}_{c}\,\left[\vec{D}_1,  \vec{D}_2,  \vec{D}_3\right]\right).
\end{equation}	
Finally, we can state
\begin{equation}
\skewsym\big(\left[\vec{D}_1,  \vec{D}_2,  \vec{D}_3\right]\tp\,\fib{\ten{R}}\tp\,\mtx{\ten{F}_{c}}\,\left[\vec{D}_1,  \vec{D}_2,  \vec{D}_3\right]\big)=
\left[\vec{D}_1,  \vec{D}_2,  \vec{D}_3\right]\tp\, \skewsym(\fib{\ten{R}}\tp\,\mtx{\ten{F}_{c}}) \,\left[\vec{D}_1,  \vec{D}_2,  \vec{D}_3\right],
\end{equation}	
i.e.,\ we have to enforce that $\skewsym(\fib{\ten{R}}\tp\,\mtx{\ten{F}_{c}})$ is zero. Note that this is equivalent to the formulation considered in \cite{simo1992h}.
