# Supplementary material for: Multidimensional coupling: A variationally consistent approach to fiber-reinforced materials
Source: arXiv:2101.02527 source file (2021-04-10)
Supplement: Supplementary file 3 [file sec_appendix0.tex]

\begin{comment}


\section{Proofs}\label{app:Axial}


%%%%%%%%%%%%%%%%%%%%%%%%%%%%%%%%%%%%%%%%%%%%%%%%%%%%%%%%%%%%%%%%%%%%%%%%%%%%%%%%%%%%%%%%%%%%

\subsection{Surface terms}\label{app:surface}

The internal virtual work reads
\begin{equation}
\delta\Pi^{int}(\vec{\varphi}) = \int\limits_{\Omega_0}\left(\vec{P}:\nabla\delta\vec{\varphi} + \mathfrak{P}\,\vdots\,\nabla^2\delta\vec{\varphi}\right)\d V.
\end{equation}
\review{Using the product rule, we obtain}
\begin{equation}
\delta\Pi^{int}(\vec{\varphi}) = \int\limits_{\Omega_0}\bigl(-\review{\left(\nabla\cdot\vec{P}\right)}\cdot\delta\vec{\varphi} + \nabla\cdot(\vec{P}\tp\,\delta\vec{\varphi})-
\nabla\cdot\mathfrak{P}:\nabla\delta\vec{\varphi} +\nabla\cdot(\mathfrak{P}\tp:\nabla\delta\vec{\varphi})\bigr) \d V,
\end{equation}
and in the second step
\begin{equation}
\delta\Pi^{int}(\vec{\varphi}) = \int\limits_{\Omega_0}\bigl(\nabla\cdot(\nabla\cdot\mathfrak{P}-\vec{P})\cdot\delta\vec{\varphi} +
\nabla\cdot[(\vec{P}\tp-\nabla\cdot\mathfrak{P}\tp)\,\delta\vec{\varphi}] + \nabla\cdot(\mathfrak{P}\tp:\nabla\delta\vec{\varphi})\bigr)\d V.
\end{equation}
Application of the divergence theorem on the second and third term yields
\begin{equation}
\delta\Pi^{int}(\vec{\varphi}) = \int\limits_{\Omega_0}\nabla\cdot(\nabla\cdot\mathfrak{P}-\vec{P})\cdot\delta\vec{\varphi}\d V +
\int\limits_{\partial\Omega_0}\bigl(\delta\vec{\varphi}\cdot[(\vec{P}-\nabla\cdot\mathfrak{P})\,\vec{N}] + \nabla\delta\vec{\varphi}:(\mathfrak{P}\,\vec{N})\bigr)\d A.
\end{equation}
Next, we decompose the last term as follows
\begin{equation}
\begin{aligned}
\nabla\delta\vec{\varphi}:(\mathfrak{P}\,\vec{N}) =\,& \nabla\cdot(\delta\vec{\varphi}\,\mathfrak{P}\,\vec{N}) - \delta\vec{\varphi}\cdot\nabla\cdot(\mathfrak{P}\,\vec{N})\\
=\,& \nabla_{\bot}\cdot(\delta\vec{\varphi}\,\mathfrak{P}\,\vec{N}) + \nabla_{\|}\cdot(\delta\vec{\varphi}\,\mathfrak{P}\,\vec{N}) \\
&- \delta\vec{\varphi}\cdot\nabla_{\bot}\cdot(\mathfrak{P}\,\vec{N})- \delta\vec{\varphi}\cdot\nabla_{\|}\cdot(\mathfrak{P}\,\vec{N}).
\end{aligned}
\end{equation}
Using the identity $\nabla_{\bot}\cdot(\delta\vec{\varphi}\,\mathfrak{P}\,\vec{N}) = \delta\vec{\varphi}\cdot\nabla_{\bot}\cdot(\mathfrak{P}\,\vec{N}) + 
\nabla_{\bot}\delta\vec{\varphi}:(\mathfrak{P}\,\vec{N})$ and the divergence theorem:
\begin{equation}
\int\limits_{\partial\Omega_0}\nabla_{\|}\cdot(\delta\vec{\varphi}\,\mathfrak{P}\,\vec{N})\d A
=\int\limits_{\partial^2\Omega_0}(\delta\vec{\varphi}\,\mathfrak{P}\,\vec{N})\cdot\hat{\vec{N}}\d S-\int\limits_{\partial\Omega_0}K\,(\delta\vec{\varphi}\,\mathfrak{P}\,\vec{N})\,\cdot\vec{N}\d A,
\end{equation}
we obtain
\begin{equation}
\begin{aligned}
\int\limits_{\partial\Omega_0} \nabla\delta\vec{\varphi}:(\mathfrak{P}\,\vec{N})\d A =
&-\int\limits_{\partial\Omega_0}\delta\vec{\varphi}\cdot(K\,(\mathfrak{P}\,\vec{N})\,\vec{N}+\nabla_{\|}\cdot(\mathfrak{P}\,\vec{N}))  - \nabla_{\bot}\delta\vec{\varphi}:\left(\mathfrak{P}\,\vec{N}\right)\d A \\ 
&+\int\limits_{\partial^2\Omega_0}\delta\vec{\varphi}\cdot(\mathfrak{P}:[\hat{\vec{N}}\otimes\vec{N}])\d S,
\end{aligned}
\end{equation}
\review{for a sufficiently smooth $\Omega_0$.}

%%%%%%%%%%%%%%%%%%%%%%%%%%%%%%%%%%%%%%%%%%%%%%%%%%%%%%%%%%%%%%%%%%%%%%%%%%%%%%%%%%%%%%%%%%%%


\subsection{Deformation gradient of the beam}\label{app:def_grad_beam}
The deformation gradient of the beam (\ref{def_grad_beam}) is given here once again:
\begin{equation}\label{app:eq_def_grad_beam}
\tilde{\vec{F}} = \tilde{\vec{\varphi}}^{\prime}\otimes\vec{D}_3 + \vec{d}_{\alpha}\otimes\vec{D}_{\alpha} + \theta^{\alpha}\,\vec{d}_{\alpha}^{\prime}\otimes\vec{D}_3.
\end{equation}
The next step is to multiply the deformation gradient with the identity matrix and to substitute the product $\vec{d}_{\alpha}\otimes\vec{D}_{\alpha}$: 
\begin{equation}
\tilde{\vec{R}}\,\tilde{\vec{R}}\tp=\tilde{\vec{R}}\tp\,\tilde{\vec{R}} = \vec{I},\qquad\qquad
\vec{d}_{\alpha}\otimes\vec{D}_{\alpha}=\tilde{\vec{R}}-\vec{d}_{3}\otimes\vec{D}_{3}.
\end{equation}
Furthermore, we use $\tilde{\vec{R}}\tp\,\vec{d}_{\alpha}^{\prime} = \tilde{\vec{R}}\tp\,\tilde{\vec{R}}^{\prime}\,\vec{D}_{\alpha}$ and $\vec{D}_{3}=\tilde{\vec{R}}\tp\,\vec{d}_3$ such that (\ref{app:eq_def_grad_beam}) ends up in:
\begin{equation}
\begin{aligned}
\tilde{\vec{F}} &= \tilde{\vec{R}}\,\left(\tilde{\vec{R}}\tp\,\tilde{\vec{\varphi}}^{\prime}\otimes\vec{D}_3 + \tilde{\vec{R}}\tp\left(\tilde{\vec{R}}-\vec{d}_{3}\otimes\vec{D}_{3}\right) + \theta^{\alpha}\,\tilde{\vec{R}}\tp\,\tilde{\vec{R}}^{\prime}\,\vec{D}_{\alpha}\otimes\vec{D}_3\right),\\
&= \tilde{\vec{R}}\,\Bigl(\underbrace{\left[\tilde{\vec{R}}\tp\,\tilde{\vec{\varphi}}^{\prime}-\vec{D}_{3}\right]}_{\vec{\Gamma}}\otimes\,\vec{D}_3  + \theta^{\alpha}\,\underbrace{\tilde{\vec{R}}\tp\,\tilde{\vec{R}}^{\prime}}_{\left[\vec{K}\right]_\times}\,\vec{D}_{\alpha}\otimes\vec{D}_3+\vec{I}\Bigr).
\end{aligned}
\end{equation}
%%%%%%%%%%%%%%%%%%%%%%%%%%%%%%%%%%%%%%%%%%%%%%%%%%%%%%%%%%%%%%%%%%%%%%%%%%%%%%%%%%%%%%%%%%%%
\subsection{Virtual work of the beam}\label{app:virt_work_beam}

 To consider again the principle of virtual work, we introduce the internal virtual work of the beam
\begin{equation}\label{eq:virt_work_beam}
\delta\tilde{\Pi}^{int} = \int\limits_{\mathfrak{C}_0}\tilde{\vec{N}}\cdot\delta\vec{\Gamma} + \tilde{\vec{M}}\cdot\delta\vec{K}\d s
\end{equation}
with the variations of the beam strain measures:
\begin{equation}\label{delta_Gamma}
\begin{aligned}
\delta\vec{\Gamma} &= \delta\left(\tilde{\vec{R}}\tp\,\tilde{\vec{\varphi}}^{\prime}-\vec{D}_{3}\right)\\
&= \delta\tilde{\vec{R}}\tp\,\tilde{\vec{\varphi}}^{\prime} +\tilde{\vec{R}}\tp\,\delta\tilde{\vec{\varphi}}^{\prime} \\
&=-\tilde{\vec{R}}\tp\,\left[\delta\vec{\phi}\right]_\times\tilde{\vec{\varphi}}^{\prime} +\tilde{\vec{R}}\tp\,\delta\tilde{\vec{\varphi}}^{\prime} \\
\end{aligned}
\end{equation}
and
\begin{equation}
\begin{aligned}
\left[\delta\vec{K}\right]_\times  &=\delta \left(\tilde{\vec{R}}\tp\,\tilde{\vec{R}}^{\prime}\right)\\
&= \delta\tilde{\vec{R}}\tp\,\tilde{\vec{R}}^{\prime}+\tilde{\vec{R}}\tp\,\delta\tilde{\vec{R}}^{\prime}\\
&= -\tilde{\vec{R}}\tp\,\left[\delta\vec{\phi}\right]_\times\tilde{\vec{R}}^{\prime}+\tilde{\vec{R}}\tp\left(\left[\delta\vec{\phi}\right]_\times\tilde{\vec{R}}\right)^\prime\\
&=\tilde{\vec{R}}\tp\left[\delta\vec{\phi}^\prime\right]_\times\tilde{\vec{R}}\\
&=-\epsilon_{ijk}\,\delta\phi^\prime_k\,\vec{D}_i\otimes\vec{D}_j,
\end{aligned}
\end{equation}
where we make use of the skew-symmetric matrix $\left[\delta\vec{\phi}^\prime\right]_\times$, which is given by:
\begin{equation}
\left[\delta\vec{\phi}^\prime\right]_\times=-\epsilon_{ijk}\,\delta\phi^\prime_k\,\vec{d}_i\otimes\vec{d}_j.
\end{equation}
The axial vector of $\left[\delta\vec{K}\right]_\times$ is then given by:
\begin{equation}\label{delta_K}
\begin{aligned}
\left[\delta\vec{K}\right] &=-\frac{1}{2}\,\epsilon_{pij}\left(-\epsilon_{ijk}\,\delta\phi^\prime_k\right) \vec{D}_p\\
&=\delta_{pk}\,\delta\phi^\prime_k\,\vec{D}_p\\
&=\tilde{\vec{R}}\tp\,\delta\vec{\phi}^\prime
\end{aligned}
\end{equation}
Inserting (\ref{delta_Gamma}) and (\ref{delta_K}) into the internal virtual work (\ref{eq:virt_work_beam}), we get:
\begin{equation}
\delta\tilde{\Pi}^{int} = \int\limits_{\mathfrak{C}_0}\left(\fib{\ten{R}}\,\fib{\ten{N}}\right)\cdot\delta\tilde{\vec{\varphi}}^{\prime} 
- \left(\fib{\vec{\varphi}}^\prime \times \fib{\ten{R}}\,\fib{\ten{N}}\right)\cdot\delta\vct{\phi}
+ \left(\fib{\ten{R}}\,\fib{\ten{M}}\right)\cdot\delta\vct{\phi}^\prime\d s,
\end{equation}
where we used once again the relation $\left[\left[\delta\vec{\phi}\right]_\times\right]_{jk}= -\epsilon_{jkl}\,\delta\vec{\phi}_l$. Here, $\mathfrak{C}_0 = [0,\,L]\subset\mathbb{R}$ and $\delta\vec{\phi}\in\mathbb{R}^3$ are the virtual rotations. 


%%%%%%%%%%%%%%%%%%%%%%%%%%%%%%%%%%%%%%%%%%%%%%%%%%%%%%%%%%%%%%%%%%%%%%%%%%%%%%%%%%%%%%%%%%%%

\end{comment}


\begin{comment}
	\section{Derivative of the terms in (\ref{eq:shortcuts})}\label{app:derivativeP}
	
	With regard to \eqref{eq:shortcuts}$_1$, we write
	\begin{equation}
	\ten{\mathcal{P}}_1^{\prime} = \frac{1}{2}\left(\vec{d}_2^{\prime}\otimes\vec{d}_3 + \vec{d}_2\otimes\vec{d}_3^{\prime}\right) -\left(\vec{d}_3^{\prime}\otimes\vec{d}_2 + \vec{d}_3\otimes\vec{d}_2^{\prime}\right).
	\end{equation}
	Noting that $\vec{d}_i^{\prime} = \tilde{\vec{R}}^{\prime}\vec{D}_i = \tilde{\vec{R}}^{\prime}\tilde{\vec{R}}^T\vec{d}_i$, where $\tilde{\vec{R}}^{\prime}\tilde{\vec{R}}^T$ is skew symmetric, such that we can define $\vec{\kappa} = \axl(\tilde{\vec{R}}^{\prime}\tilde{\vec{R}}^T)$. Thus, we obtain
	\begin{equation}
	\begin{aligned}
	\ten{\mathcal{P}}_1^{\prime} &= \frac{1}{2}\left(\VPTen{\vec{\kappa}}\vec{d}_2\otimes\vec{d}_3 + \vec{d}_2\otimes\VPTen{\vec{\kappa}}\vec{d}_3\right) - 
	\left(\VPTen{\vec{\kappa}}\vec{d}_3\otimes\vec{d}_2 + \vec{d}_3\otimes\VPTen{\vec{\kappa}}\vec{d}_2\right),\\
	&= \frac{1}{2}\left(\VPTen{\vec{\kappa}}\vec{d}_2\otimes\vec{d}_3 - \vec{d}_2\otimes\vec{d}_3\VPTen{\vec{\kappa}}\right) - 
	\left(\VPTen{\vec{\kappa}}\vec{d}_3\otimes\vec{d}_2 - \vec{d}_3\otimes\vec{d}_2\VPTen{\vec{\kappa}}\right),\\
	&= \VPTen{\vec{\kappa}}\ten{\mathcal{P}}_1 - \ten{\mathcal{P}}_1\VPTen{\vec{\kappa}}.
	\end{aligned}
	\end{equation}
	All further terms presented in \eqref{eq:shortcuts}$_2$ follow analoguesly.
\end{comment}
